# Supplementary material for: Optimization-Induced Dynamics of Lipschitz Continuity in Neural Networks
Source: arXiv:2506.18588 source file (2025-11-14)
Supplement: Supplementary file 1 [file appendix_system_entropy_production.tex]

\section{System Entropy Production}

\begin{proposition}[System Entropy Production]
By viewing $Z(t)$ as a system state, the Fokker-Plank Equation (FPE) can give the distribution of $Z(t)$ as $p(Z,t)$. At a $t$, the Shannon entropy of $Z(t)$ is given by:
\begin{align}
    S(Z,t) := -\int p(Z,t) \,\log{p(Z,t)} \;\dd Z(t),
\end{align}
and similarly define:
\begin{align}
   S(K,t) := -\int p(K,t) \,\log{p(K,t)} \;\dd K(t). 
\end{align}

Then, the entropy production of $S(K ,t)$ is given as:
\begin{align}
\frac{\mathrm{d} S(K, t)}{\mathrm{d} t} = \frac{\mathrm{d} S(Z, t)}{\mathrm{d} t} + \mathbb{E}[\mu_Z(t) + \kappa_Z(t) - \frac{1}{2} \lambda_Z(t)^2],
\end{align}
where the $\boldsymbol{\kappa}(t)$ contributes to the non-negative, irreversible increments of the system entropy, arising from the interaction between operator-norm curvature and gradient noise arising from mini-batch sampling. 

\end{proposition}

\subsection{Setting for Analysis}
Define:
\begin{align}
b(t, Z^{(\ell)}) = \boldsymbol{\mu}^{(\ell)}(t) + \boldsymbol{\kappa}^{(\ell)}(t), \quad D(t, Z^{(\ell)}) = \frac{1}{2} \|\boldsymbol{\lambda}^{(\ell)}(t)\|_2^2.
\end{align}

\subsection{Fokker-Planck Equation for $Z^{(\ell)}(t)$}
The SDE is:
\begin{align}
\mathrm{d} Z^{(\ell)}(t) = b(t, Z^{(\ell)}) \mathrm{d} t + \sqrt{2 D(t, Z^{(\ell)})} \mathrm{d} B_t,
\end{align}
where $\sqrt{2 D(t, Z^{(\ell)})} = \|\boldsymbol{\lambda}^{(\ell)}(t)\|_2$. The FPE is:
\begin{align}
\frac{\partial p(Z^{(\ell)}, t)}{\partial t} = -\frac{\partial}{\partial Z^{(\ell)}} \left[ b(t, Z^{(\ell)}) p(Z^{(\ell)}, t) \right] + \frac{\partial^2}{\partial {Z^{(\ell)}}^2} \left[ D(t, Z^{(\ell)}) p(Z^{(\ell)}, t) \right].
\end{align}

To simplify, denote $p = p(Z^{(\ell)}, t)$:
\begin{align}
\frac{\partial p}{\partial t} = -\frac{\partial}{\partial Z^{(\ell)}} \left[ \left( \boldsymbol{\mu}^{(\ell)}(t) + \boldsymbol{\kappa}^{(\ell)}(t) \right) p \right] + \frac{\partial^2}{\partial {Z^{(\ell)}}^2} \left[ \frac{1}{2} \|\boldsymbol{\lambda}^{(\ell)}(t)\|_2^2 p \right].
\end{align}

\subsection{Entropy of $Z^{(\ell)}(t)$}
The Shannon entropy is:
\begin{align}
S(Z^{(\ell)}, t) = -\int p(Z^{(\ell)}, t) \log p(Z^{(\ell)}, t) \mathrm{d} Z^{(\ell)}.
\end{align}
The entropy production rate is:
\begin{align}
\frac{\mathrm{d} S(Z^{(\ell)}, t)}{\mathrm{d} t} = -\int \left[ \log p(Z^{(\ell)}, t) + 1 \right] \frac{\partial p(Z^{(\ell)}, t)}{\partial t} \mathrm{d} Z^{(\ell)}.
\end{align}
Substitute the FPE:
\begin{align}
\frac{\mathrm{d} S}{\mathrm{d} t} = -\int \left( \log p + 1 \right) \left[ -\frac{\partial}{\partial Z^{(\ell)}} \left( b(t, Z^{(\ell)}) p \right) + \frac{\partial^2}{\partial {Z^{(\ell)}}^2} \left( D(t, Z^{(\ell)}) p \right) \right] \mathrm{d} Z^{(\ell)}.
\end{align}

\subsubsection{Drift Term}
Compute:
\begin{align}
\int \left( \log p + 1 \right) \frac{\partial}{\partial Z^{(\ell)}} \left( b(t, Z^{(\ell)}) p \right) \mathrm{d} Z^{(\ell)} = \int \log p \frac{\partial}{\partial Z^{(\ell)}} (b p) \mathrm{d} Z^{(\ell)} + \int \frac{\partial}{\partial Z^{(\ell)}} (b p) \mathrm{d} Z^{(\ell)}.
\end{align}

\paragraph{Second term.} For the second term:
\begin{align}
\int_{-\infty}^{\infty} \frac{\partial}{\partial Z^{(\ell)}} (b p) \mathrm{d} Z^{(\ell)} = \left[ b(t, Z^{(\ell)}) p(Z^{(\ell)}, t) \right]_{-\infty}^{\infty}.
\end{align}

Since $p(Z^{(\ell)}, t)$ is a probability density, it satisfies
\begin{align}
  \int_{-\infty}^{\infty} p(Z^{(\ell)}, t) \mathrm{d} Z^{(\ell)} = 1
  ,
\end{align}
and typically decays as $Z^{(\ell)} \to \pm \infty$. 

Note $b(t, Z^{(\ell)}) = \frac{c_1(t) + c_2(t)}{e^{Z^{(\ell)}}}$:
\begin{enumerate}
    \item As $Z^{(\ell)} \to \infty$, $e^{Z^{(\ell)}} \to \infty$, so $b(t, Z^{(\ell)}) \to 0$. If $p(Z^{(\ell)}, t)$ decays faster than $e^{Z^{(\ell)}}$ grows, $b p \to 0$.

    \item  As $Z^{(\ell)} \to -\infty$, $e^{Z^{(\ell)}} \to 0$, so $b(t, Z^{(\ell)}) \to \infty$. 
\end{enumerate}

Since $K^{(\ell)}(t) = e^{Z^{(\ell)}} > 0$, $p(Z^{(\ell)}, t)$ has negligible mass for large negative $Z^{(\ell)}$, ensuring $b p \to 0$. Thus:
\begin{align}
\left[ b(t, Z^{(\ell)}) p(Z^{(\ell)}, t) \right]_{-\infty}^{\infty} = 0.
\end{align}

\paragraph{First term.} First term:
\begin{align}
\int \log p \frac{\partial}{\partial Z^{(\ell)}} (b p) \mathrm{d} Z^{(\ell)} = \left[ \log p \cdot b p \right]_{-\infty}^{\infty} - \int b p \frac{\partial \log p}{\partial Z^{(\ell)}} \mathrm{d} Z^{(\ell)} = -\int b \frac{\partial p}{\partial Z^{(\ell)}} \mathrm{d} Z^{(\ell)}.
\end{align}
\begin{align}
-\int b \frac{\partial p}{\partial Z^{(\ell)}} \mathrm{d} Z^{(\ell)} = -\left[ b p \right]_{-\infty}^{\infty} + \int p \frac{\partial b}{\partial Z^{(\ell)}} \mathrm{d} Z^{(\ell)} = \int p \left( -b \right) \mathrm{d} Z^{(\ell)} = -\mathbb{E}[b(t, Z^{(\ell)})].
\end{align}
Thus:
\begin{align}
-\int \left( \log p + 1 \right) \frac{\partial}{\partial Z^{(\ell)}} (b p) \mathrm{d} Z^{(\ell)} = \mathbb{E}[b(t, Z^{(\ell)})].
\end{align}

\subsubsection{Diffusion Term}
Compute:
\begin{align}
\int \left( \log p + 1 \right) \frac{\partial^2}{\partial {Z^{(\ell)}}^2} \left( D(t, Z^{(\ell)}) p \right) \mathrm{d} Z^{(\ell)} = \int \log p \frac{\partial^2}{\partial {Z^{(\ell)}}^2} (D p) \mathrm{d} Z^{(\ell)} + \int \frac{\partial^2}{\partial {Z^{(\ell)}}^2} (D p) \mathrm{d} Z^{(\ell)}.
\end{align}

Second term:
\begin{align}
\int \frac{\partial^2}{\partial {Z^{(\ell)}}^2} (D p) \mathrm{d} Z^{(\ell)} = \left[ \frac{\partial (D p)}{\partial Z^{(\ell)}} \right]_{-\infty}^{\infty} = 0.
\end{align}

First term:
\begin{align}
\int \log p \frac{\partial^2}{\partial {Z^{(\ell)}}^2} (D p) \mathrm{d} Z^{(\ell)} = \left[ \log p \frac{\partial (D p)}{\partial Z^{(\ell)}} \right]_{-\infty}^{\infty} - \int \frac{\partial \log p}{\partial Z^{(\ell)}} \frac{\partial (D p)}{\partial Z^{(\ell)}} \mathrm{d} Z^{(\ell)}.
\end{align}

Compute:
\begin{align}
D(t, Z^{(\ell)}) = \frac{1}{2} \|\boldsymbol{\lambda}^{(\ell)}(t)\|_2^2 = \frac{\eta}{2 e^{2 Z^{(\ell)}}} \boldsymbol{J}_{\mathrm{op}}^{(\ell)}(t)^\top \boldsymbol{\Sigma}_t^{(\ell)} \boldsymbol{J}_{\mathrm{op}}^{(\ell)}(t).
\end{align}

Let $d(t) = \frac{\eta}{2} \boldsymbol{J}_{\mathrm{op}}^{(\ell)}(t)^\top \boldsymbol{\Sigma}_t^{(\ell)} \boldsymbol{J}_{\mathrm{op}}^{(\ell)}(t)$:
\begin{align}
D(t, Z^{(\ell)}) = \frac{d(t)}{e^{2 Z^{(\ell)}}}, \quad \frac{\partial D}{\partial Z^{(\ell)}} = -\frac{2 d(t)}{e^{2 Z^{(\ell)}}} = -2 D(t, Z^{(\ell)}).
\end{align}
\begin{align}
\frac{\partial (D p)}{\partial Z^{(\ell)}} = D \frac{\partial p}{\partial Z^{(\ell)}} + p \frac{\partial D}{\partial Z^{(\ell)}} = D \frac{\partial p}{\partial Z^{(\ell)}} - 2 D p.
\end{align}
\begin{align}
\frac{\partial^2}{\partial {Z^{(\ell)}}^2} (D p) &= \frac{\partial}{\partial Z^{(\ell)}} \left( D \frac{\partial p}{\partial Z^{(\ell)}} - 2 D p \right) \\
&= D \frac{\partial^2 p}{\partial {Z^{(\ell)}}^2} - 2 \frac{\partial D}{\partial Z^{(\ell)}} \frac{\partial p}{\partial Z^{(\ell)}} - 2 D \frac{\partial p}{\partial Z^{(\ell)}} + p \frac{\partial^2 D}{\partial {Z^{(\ell)}}^2} - 2 \frac{\partial D}{\partial Z^{(\ell)}} p.
\end{align}
\begin{align}
\frac{\partial^2 D}{\partial {Z^{(\ell)}}^2} = \frac{\partial}{\partial Z^{(\ell)}} (-2 D) = -2 \frac{\partial D}{\partial Z^{(\ell)}} = 4 D.
\end{align}
\begin{align}
\frac{\partial^2}{\partial {Z^{(\ell)}}^2} (D p) = D \frac{\partial^2 p}{\partial {Z^{(\ell)}}^2} - 4 D \frac{\partial p}{\partial Z^{(\ell)}} + 4 D p.
\end{align}

Thus:
\begin{align}
\int \log p \frac{\partial^2}{\partial {Z^{(\ell)}}^2} (D p) \mathrm{d} Z^{(\ell)} = \int \log p \left( D \frac{\partial^2 p}{\partial {Z^{(\ell)}}^2} - 4 D \frac{\partial p}{\partial Z^{(\ell)}} + 4 D p \right) \mathrm{d} Z^{(\ell)}.
\end{align}

Split:
\begin{align}
\int \log p D \frac{\partial^2 p}{\partial {Z^{(\ell)}}^2} \mathrm{d} Z^{(\ell)} &= \left[ \log p D \frac{\partial p}{\partial Z^{(\ell)}} \right]_{-\infty}^{\infty} - \int \frac{\partial \log p}{\partial Z^{(\ell)}} D \frac{\partial p}{\partial Z^{(\ell)}} \mathrm{d} Z^{(\ell)} \notag \\
&\qquad -\int \log p \frac{\partial D}{\partial Z^{(\ell)}} \frac{\partial p}{\partial Z^{(\ell)}} \mathrm{d} Z^{(\ell)}.
\end{align}
\begin{align}
-4 \int \log p D \frac{\partial p}{\partial Z^{(\ell)}} \mathrm{d} Z^{(\ell)} = -4 \left[ \log p D p \right]_{-\infty}^{\infty} + 4 \int p D \frac{\partial \log p}{\partial Z^{(\ell)}} \mathrm{d} Z^{(\ell)} + 4 \int \log p \frac{\partial D}{\partial Z^{(\ell)}} p \mathrm{d} Z^{(\ell)}.
\end{align}
\begin{align}
4 \int \log p D p \mathrm{d} Z^{(\ell)} = 4 \mathbb{E}[\log p D].
\end{align}

Combine:
\begin{align}
\frac{\mathrm{d} S}{\mathrm{d} t} = \mathbb{E}[b(t, Z^{(\ell)})] - \mathbb{E}\left[ D(t, Z^{(\ell)}) \left( \frac{1}{p} \frac{\partial p}{\partial Z^{(\ell)}} \right)^2 \right] - \mathbb{E}\left[ \frac{2 D(t, Z^{(\ell)})}{p} \frac{\partial p}{\partial Z^{(\ell)}} \right] + 4 \mathbb{E}[D(t, Z^{(\ell)})].
\end{align}

\subsection{Entropy of $K^{(\ell)}(t)$}
\begin{align}
p(K^{(\ell)}, t) = \frac{p(Z^{(\ell)}, t)}{K^{(\ell)}}.
\end{align}
\begin{align}
S(K^{(\ell)}, t) &= -\int p(Z^{(\ell)}, t) \left[ \log p(Z^{(\ell)}, t) - \log K^{(\ell)} \right] \mathrm{d} Z^{(\ell)} \\
&= S(Z^{(\ell)}, t) + \mathbb{E}[Z^{(\ell)}(t)].
\end{align}
\begin{align}
\mathbb{E}[Z^{(\ell)}(t)] = Z^{(\ell)}(0) + \int_0^t \mathbb{E}[\boldsymbol{\mu}^{(\ell)}(s) + \boldsymbol{\kappa}^{(\ell)}(s)] \mathrm{d} s.
\end{align}
\begin{align}
\frac{\mathrm{d} S(K^{(\ell)}, t)}{\mathrm{d} t} = \frac{\mathrm{d} S(Z^{(\ell)}, t)}{\mathrm{d} t} + \mathbb{E}[\boldsymbol{\mu}^{(\ell)}(t) + \boldsymbol{\kappa}^{(\ell)}(t)].
\end{align}

Since $\boldsymbol{\kappa}^{(\ell)}(t) \geq 0$, it contributes positively. Near convergence, $\boldsymbol{\mu}^{(\ell)}(t) \approx 0$, $\boldsymbol{\lambda}^{(\ell)}(t) \to \boldsymbol{0}$, so $\mathbb{E}[\boldsymbol{\kappa}^{(\ell)}(t)]$ dominates, driving irreversible entropy increases.

\subsection{Network-Level Entropy}
For $K(t) = e^{Z(t)}$:
\begin{align}
\mathrm{d} Z(t) = \left( \mu_Z(t) + \kappa_Z(t) - \frac{1}{2} \lambda_Z(t)^2 \right) \mathrm{d} t + \lambda_Z(t) \mathrm{d} W_t,
\end{align}
\begin{align}
\frac{\mathrm{d} S(K, t)}{\mathrm{d} t} = \frac{\mathrm{d} S(Z, t)}{\mathrm{d} t} + \mathbb{E}[\mu_Z(t) + \kappa_Z(t) - \frac{1}{2} \lambda_Z(t)^2].
\end{align}
Near convergence, $\kappa_Z(t)$ drives irreversible entropy increases.

\subsection{Discussions}
\begin{enumerate}
    \item $\boldsymbol{\mu}^{(\ell)}(t)$: Affects $\mathbb{E}[Z^{(\ell)}(t)]$, contributing variably; negligible near convergence.
    
    \item $\boldsymbol{\kappa}^{(\ell)}(t)$: Drives irreversible entropy increases.
    
    \item $\boldsymbol{\lambda}^{(\ell)}(t)$: Affects diffusion; diminishes near convergence.
\end{enumerate}
